# Supplementary material for: DRIM: Learning Disentangled Representations from Incomplete Multimodal Healthcare Data
Source: arXiv:2409.17055 source file (2024-10-01)
Supplement: Supplementary file 1 [file supplemental.pdf]

# Supplementary material

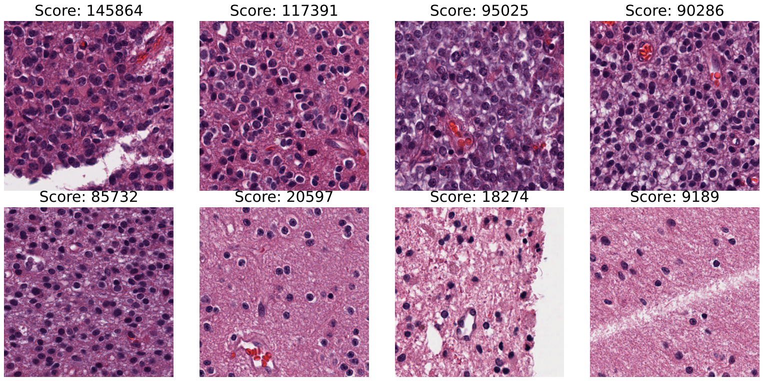


Fig. S1: Random patches with scores based on the number of pixels meeting these conditions: saturation > 150 and value < 150 in HSV space.

Table S1: Comparison of trainable parameters across fusion functions.

| Fusion | N modalities | Representation size | Parameters (in millions) |
|---|---|---|---|
| MAFusion | 4 | 32 | 0.14 |
| | | 128 | 0.56 |
| | 5 | 32 | 0.14 |
| | | 128 | 0.56 |
| Tensor | 4 | 32 | 38.10 |
| | | 128 | ∼34500 |
| | 5 | 32 | 1252.51 |
| | | 128 | ∼4390000 |

Table S2: Experiments from this study were run on a desktop machine (AMD EPYC 7502P 32-Core Processor, 64 GB RAM) with NVIDIA GeForce 2080 Ti.

| Task | Mode | $N$ GPUs | Time by experiment |
|---|---|---|---|
| Pretraining | WSI | 4 | ∼ 16 hours |
| | MRI | 4 | ∼ 30 min |
| Survival | All but Tensor | 1 | ∼ 9 min |
| | Tensor | 1 | ∼ 12 min |
| | DRIM-Surv | 1 | ∼ 10 min |
| | DRIM-U | 1 | ∼ 13 min |

Table S3: Sensitivity analysis over the $\gamma$ coefficient. Performance metrics for models using solely shared encoders and for the DRIM-Surv model without the $\mathcal{L}_{sh}$ term (indicated as 0 in the table) is also displayed.

| Sensitivity ($\mathcal{L}_{sh}$, $\gamma$) | C-index (↑) | Integrated BS (↓) | INBLL (↓) |
|---|---|---|---|
| (1, -) | 0.750 ± 0.016 | 0.090 ± 0.006 | 0.324 ± 0.022 |
| (0., 0.) | 0.741 ± 0.007 | 0.090 ± 0.006 | 0.324 ± 0.027 |
| (1., 0.) | 0.733 ± 0.013 | 0.091 ± 0.006 | 0.339 ± 0.040 |
| (1., 0.1) | 0.754 ± 0.013 | 0.089 ± 0.009 | 0.307 ± 0.053 |
| (1., 0.2) | 0.759 ± 0.014 | 0.094 ± 0.006 | 0.312 ± 0.034 |
| (1., 0.3) | 0.752 ± 0.017 | 0.094 ± 0.009 | 0.329 ± 0.055 |
| (1., 0.4) | 0.762 ± 0.009 | 0.093 ± 0.005 | 0.311 ± 0.015 |
| (1., 0.5) | 0.761 ± 0.011 | 0.091 ± 0.003 | 0.302 ± 0.016 |
| (1., 0.6) | 0.767 ± 0.009 | 0.092 ± 0.004 | 0.307 ± 0.025 |
| (1.,0.7) | 0.768 ± 0.005 | 0.090 ± 0.005 | 0.299 ± 0.023 |
| (1., 0.8) | 0.774 ± 0.006 | 0.086 ± 0.004 | 0.285 ± 0.016 |
| (1., 0.9) | 0.774 ± 0.013 | 0.090 ± 0.005 | 0.298 ± 0.021 |
| (1., 1.) | 0.758 ± 0.008 | 0.091 ± 0.004 | 0.300 ± 0.020 |

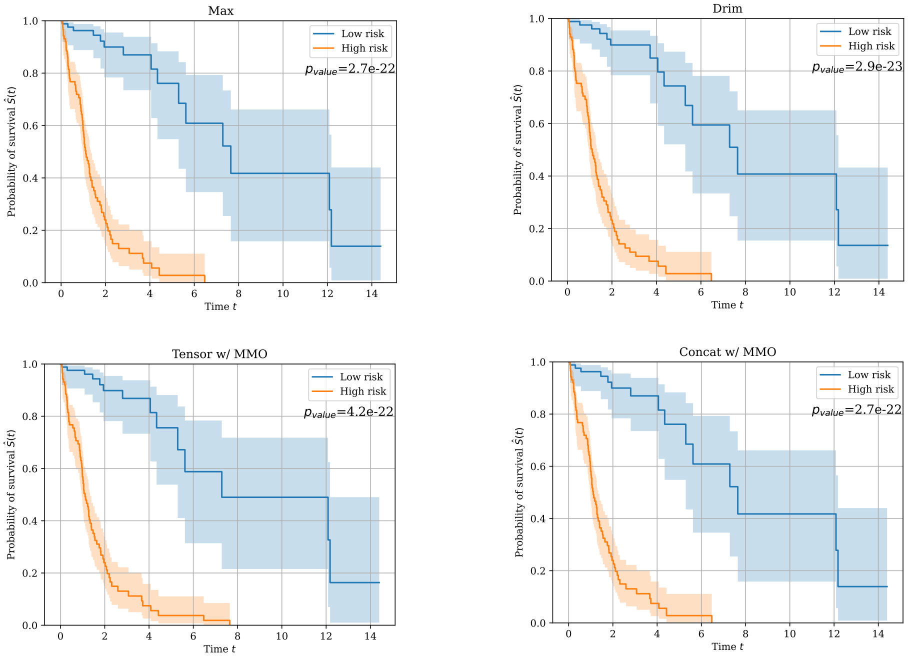


Fig. S2: Patient stratification into high-risk and low-risk categories with different survival models.
